# Supplementary material for: Comprehension and quotient structures in the language of 2-categories
Source: arXiv:2005.10015 source file (2020-05-20)
Supplement: Supplementary file 1 [file appendix.tex]

\appendix

\section{Four notions of comprehension categories}

\subsection{Comprehension categories.} As defined by Jacobs (\cite{jacobs-paper}, p. 181, and \cite{jacobs:book}, chapter 10.4, page 613)
A comprehension category is a fibration 
$p:\catE\to \catB$ equipped with
functor $comp:\catE\to \catBarr$ such that $cod \compose \composeH comp = p $, 
where $cod : \catBArr \to \catB$ is the codomain functor , and transporting every $p$-cartesian morphism of $\catE$
to a $\cod$-cartesian morphism in $\catB$, that is, to \textit{pullback} squares in $\catB$.

\subsection{$D$-categories.} Introduced under the name of $D$-category by \cite{ehrhard} and called \textit{comprehension category with units} in \cite{jacobs-paper} def. 4.12. The name of Ehrhard comprehension category is given by \cite{moss2018dialectica}, p 22.
An Ehrhard comprehension category is a fibration
$p:\catE\to \catB$ equipped with a fully faithful right adjoint $s:\catB\to \catE$
which itself has a right adjoint $comp: \catE\to\catB$.

\subsection{$F$-categories.}
called $tC$-opfibration by Fumex in his PhD thesis, (\cite{fumex-phdthesis} p. 38, def. 2.2.2.)
A Fumex category is an opfibration $p:\catE\to\catB$ with a fully faithful section $\sectionp{}:\catB\to\catE$ with a right adjoint.
The fullness and faithfulness condition is equivalent to the fact that the comprehension of $\sectionp{A}$ (unit of the adjunction) is an iso.

\subsection{Lawvere categories.} 
As defined in \cite{jacobs-paper}, p 190.
It is a bifibration $p:\catE\to\catB$ with a terminal object in each fiber, defining a functor $\sectionp{}:\catB\to\catE$, and such that the (ordinary) functor
$$
f \mapsto \Sigma_f \sectionp{(dom f)} : \catBarr\to \catE
$$
induced by the left fibration structure has a right adjoint $comp:\catE\to\catBarr$, verifying $cod\circ comp=p$,
and such that the unit and counit are vertical (their image by $cod$ and $p$ is the identity).

\section{The 2-category $\Endo{\Cat}$}

We consider the sub-2-category $\EndoCat$ of $\SliceLax{\Cat}$ 
whose objects are pairs $(X,x)$ of a category $X$ and endo-functor $x: X \to X$, 
whose 1-morphisms  $(P,p) : (X,x) \to (Y,y)$ are pairs of a functor $P : X \to Y$ and a natural transformation $p : y\composeH P \naturalto P\composeH x$,
depicted in $\Cat$ as a commutative or a string diagram :
$$
\begin{array}{ccc}
\begin{tikzcd}[column sep=1.5em,row sep=1.5em]
X  \ar[dd, "{x}"'] \ar[rr,"P"] & {} & Y \ar[dd,"{y}"] 
\\
{} & {} & {} \ar[ll,shorten <>=15pt,Rightarrow, "p"',yshift=-0.5em]
\\
X   \ar[rr,"P"]  & {} & Y
\end{tikzcd}
& \quad\quad &
\begin{tikzpicture}[scale=0.6]
\begin{scope}[yscale=1,xscale=1]
\draw[name path=path1, s] 
(0,4) node[above] {$P$}
to[in=90, out=-90]  (2,0)
to[in=90, out=-90]  (2,0) node[below]{$P$};
\draw[name path=path2,t]
(2,4)  node[above] {$x$}
to[in=90, out=-90] (0,0) node[below]{$y$};
\draw[name intersections={of=path1 and path2}] (intersection-1) node[below] {$p$};
\draw[fill] (intersection-1.north) circle (.08);
\end{scope}
\end{tikzpicture}
\end{array}
$$

\noindent
Its 2-morphisms $\alpha : (P,p) \naturalto (Q,q) : (X,x) \to (Y,y)$ are made of a \emph{single} natural transformation $\alpha : P \naturalto Q$ such that 
$\alpha \composeH x \composeV p = q \composeV y \composeH \alpha$ depicted in string diagram as
\begin{equation}\label{equation/2morphendo}
\begin{array}{ccc}
\begin{tikzpicture}[scale=0.4]
\begin{scope}[yscale=1,xscale=1]
\draw[name path=path1, s] 
(0,6) node[above] {$Q$}
to (0,5)  node[left] (alpha) {$\alpha$}
to (0,4)
to[in=90, out=-90]  (2,0) node[below]{$P$};
\draw[name path=path2,t]
(2,6)  node[above] {$x$}
to (2, 4)
to[in=90, out=-90] (0,0) node[below]{$y$};
\draw[name intersections={of=path1 and path2}] (intersection-1) node[below] {$p$};
\draw[fill] (alpha.east) circle (.08);
\draw[fill] (intersection-1.north) circle (.08);
\end{scope}
\end{tikzpicture}
\quad = \quad
\begin{tikzpicture}[scale=0.4]
\begin{scope}[yscale=1,xscale=1]
\draw[name path=path1, s] 
(0,6) node[above] {$Q$}
to[in=90, out=-90] (2,2)
to[in=90, out=-90] (2,1)  node[right] (alpha) {$\alpha$}
to[in=90, out=-90]  (2,0) node[below]{$P$};
\draw[name path=path2,t]
(2,6)  node[above] {$x$}
to[in=90, out=-90] (0, 2)
to[in=90, out=-90] (0,0) node[below]{$y$};
\draw[name intersections={of=path1 and path2}] (intersection-1) node[below] {$q$};
\draw[fill] (alpha.west) circle (.08);
\draw[fill] (intersection-1.north) circle (.08);
\end{scope}
\end{tikzpicture}
\end{array}
\end{equation}

\noindent
Adjunctions $(L,l) : (X,x) \to (Y,y) \quad \vdash \quad (R,r):(Y,y) \to (X,x)$ in $\EndoCat$  amounts to an single adjunction in $\Cat$ whone unit and counit satisfy the triangular equations $\eta x  = Rl\circ rL \circ x \eta $ and $y \varepsilon = \varepsilon y \circ Lr \circ lR
$	pictured in string diagrams  below
$$
\begin{array}{cccccc}
\begin{tikzpicture}[scale=0.4]
\begin{scope}[yscale=1,xscale=1]
\draw[name path=path1, s]
(0,6) node[above] {$R$}
to[in=160, out=-90] (1,3) node[below] (eta) {$\eta$}
to[in=-90, out=20]  (2,6) node[above]{$L$};
\draw[name path=path2,t]
(3,6)  node[above] {$x$}
to (3, 4)
to[in=90, out=-90] (3,0) node[below]{$x$};
\draw[fill] (eta.north) circle (.08);
\end{scope}
\end{tikzpicture}
\quad = \quad
\begin{tikzpicture}[scale=0.4]
\begin{scope}[yscale=1,xscale=1]
\draw[name path=path1, s] 
(0,6) node[above] {$R$}
to[in=160, out=-90] (3,1)  node[below] (eta) {$\eta$};
\draw[name path=path2, s] 
(2,6) node[above] {$L$}
to[in=20, out=-90] (3,1);
\draw[fill] (eta.north) circle (.08);
\draw[name path=path3,t]
(4,6)  node[above] {$x$}
to[in=90, out=-90] (0, 2)
to[in=90, out=-90] (0,0) node[below]{$x$};
\draw[name intersections={of=path1 and path3}] (intersection-1) node[right] {$r$};
\draw[fill] (intersection-1.west) circle (.08);
\draw[name intersections={of=path2 and path3}] (intersection-1) node[right] {$l$};
\draw[fill] (intersection-1.west) circle (.08);
\end{scope}
\end{tikzpicture}
\quad \quad \quad
\begin{tikzpicture}[scale=0.4]
\begin{scope}[yscale=-1,xscale=-1]
\draw[name path=path1, s]
(0,6) node[below] {$R$}
to[in=160, out=-90] (1,3) node[above] (epsilon) {$\varepsilon$}
to[in=-90, out=20]  (2,6) node[below]{$L$};
\draw[name path=path2,t]
(3,6)  node[below] {$y$}
to (3, 4)
to[in=90, out=-90] (3,0) node[above]{$y$};
\draw[fill] (epsilon.south) circle (.08);
\end{scope}
\end{tikzpicture}
\quad = \quad
\begin{tikzpicture}[scale=0.4]
\begin{scope}[yscale=-1,xscale=-1]
\draw[name path=path1, s] 
(0,6) node[below] {$R$}
to[in=160, out=-90] (3,1)  node[above] (epsilon) {$\varepsilon$};
\draw[name path=path2, s] 
(2,6) node[below] {$L$}
to[in=20, out=-90] (3,1);
\draw[fill] (epsilon.south) circle (.08);
\draw[name path=path3,t]
(4,6)  node[below] {$y$}
to[in=90, out=-90] (0, 2)
to[in=90, out=-90] (0,0) node[above]{$y$};
\draw[name intersections={of=path1 and path3}] (intersection-1) node[right] {$r$};
\draw[fill] (intersection-1.west) circle (.08);
\draw[name intersections={of=path2 and path3}] (intersection-1) node[below] {$l$};
\draw[fill] (intersection-1.north) circle (.08);
\end{scope}
\end{tikzpicture}
\end{array}
$$

\subsection{Path-objects in $\Endo{\Cat}$}

We know that $\Cat$ has for each object $B$ the path-objects $B^{\to}$ which is its arrow category, and we can easily show that $\Endo{\Cat}$ has path-objects too.
From a given object $(B,b)$ in $\Endo{\Cat}$ we consider pair $(B^{\to},b^{\to}$ where $b^{\to}$ is the endofunctor acting on arrows of $B$ as expected, the 1-morphisms $(dom, id) : (B^{\to},b^{\to} \to (B,b)$  and $(cod, id) : (B^{\to},b^{\to} \to (B,b) $, as well as the 2-morphism $\arrowcell : (dom, id) \naturalto (cod, id) : (B^{\to},b^{\to}) \to (B,b)$ verifying that for any other 2-morphism  $\alpha : (P,p) \to (Q,q) : (X,x) \to (B,b)$ in $\Endo{\Cat}$ 

\begin{equation*}
\begin{array}{ccc}
\begin{tikzcd}[scale=0.7,column sep =3em]
(X,x)
\arrow[bend left]{rr}[name=Y]{(P,p)}
\arrow[bend right]{rr}[name=X,swap]{(Q,q)}
\arrow[ shorten <>=5pt, Leftarrow,to path={([xshift=0em]X) -- node[label=right:$\alpha$] {} ([xshift=0em]Y)}] & {} & (B,b)
\end{tikzcd}
 &= &
\begin{tikzcd}[scale=0.7,column sep =3em]
(X,x) \arrow{r}{(a,(p,q))}  & (B^{\to},b^{\to})
\arrow[bend left]{rr}[name=Y]{(dom,id)} 
\arrow[bend right]{rr}[name=X,swap]{(cod,id)}
\arrow[ shorten <>=5pt, Leftarrow,to path={([xshift=0em]X) -- node[label=right:$\arrowcell$] {} ([xshift=0em]Y)}] & {} & (B,b)
\end{tikzcd}
\end{array}
\end{equation*}

\noindent 
The natural transformation $\alpha  : P \naturalto Q$ determines a collection of arrows in $B$, and $a : X \to B^{\to}$ assembles those in a functor. It is defined thanks to universality of $\arrowcell$ in $\Cat$, by $\arrowcell \composeH a = \alpha $. We can verify that Eq (\ref{equation/2morphendo}) 
$ \alpha \composeH x \composeV p = q \composeV b \composeH \alpha $, ensures that $(p,q) : b^{\to} \composeH a \naturalto a \composeH b^{\to}$ is a natural transformation ending in $B^{\to}$ and we thus have a 1-morphism 
$(a, (q,p)) : (X,x) \to (B^{\to}, b^{\to})$ of $\Endo{\Cat}$. By inspection, we see that $(cod,id) \composeH (a,(p,q)) = (Q,q) : (X,x) \to (B,b)$ as well as  $(dom,id) \composeH (a,(p,q)) = (P,p) : (X,x) \to (B,b)$. Thus, as 2-morphisms of $\Endo{\Cat}$, we have that~$app \composeH (a, (q,p)) = \alpha : (P,p) \to (Q,q) : (X,x) \to (B,b)$ as per the picture above.

\subsection{$Alg$ from $\Endo{\Cat}$ to algebras}

Recall (cf Beck \cite{beck1969distributive}) that we can classically define the 2-functor
$$Alg = \Endo{\Cat}(1_1,\varOne) : \Endo{\Cat} \to \Cat $$ 
mapping an endofunctor to its category of algebras (cf \cite{beck1969distributive}) and $\Cod$ mapping an endofunctor to its underlying category, and dually $Clg$ mapping an endofunctor to its category of coalgebras

\begin{equation*}
\begin{array}{c}
\begin{tikzcd}[column sep =3em]
{\EndoCat}
\arrow[rr,yshift=.2em,"{Alg}"{swap,name=source,description},bend left=30] 
\arrow[rr,yshift=-.2em,"{\Cod}"{swap,name=target,description},bend right=30] 
&& 
\Cat
\arrow[from=source,to=target,double,-implies,shorten <>=2pt,"{U}"{description,pos=.5}]
\end{tikzcd}
\end{array}
\end{equation*}

\noindent
Thus any adjunction  $(L,l)  \dashv (R,r):(Y,y) \to (X,x)$ in $\Endo{\Cat}$
is tranported by this pair of 2-functors into a pair of adjunction in $\Cat$ 
$$L^l \quad  \dashv  \quad R^r : Alg(y) \to Alg(x) \quad \quad \quad \quad L \quad  \dashv  \quad R : Y \to X$$
\noindent
connected by the components of the 2-natural transformations $U$ algebras to their codomain.
